# Supplementary material for: Critical role of water in defect aggregation and chemical degradation of perovskite solar cells
Source: arXiv:1708.07606 source file (2018-03-13)
Supplement: Supplementary file 1 [file hydperov-jpcl-supp.pdf]

# Supporting information – Role of vacancy point defects and water molecule in the degradation of the halide perovskite $CH_3NH_3PbI_3$ through hydration step

Yun-Hyok Kye[a], Chol-Jun Yu[a,*], Un-Gi Jong[a,b], Yue Chen[c], and Aron Walsh[d]

[a] *Department of Computational Materials Design, Faculty of Materials Science, Kim Il Sung University, Ryongnam-Dong, Taesong District, Pyongyang, Democratic People's Republic of Korea*

[b] *Natural Science Centre, Kim Il Sung University, Ryongnam-Dong, Taesong District, Pyongyang, Democratic People's Republic of Korea*

[c] *Department of Mechanical Engineering, The University of Hong Kong, Pokfulam Road, Hong Kong SAR, China*

[d] *Department of Materials, Imperial College London, London SW7 2AZ, United Kingdom*

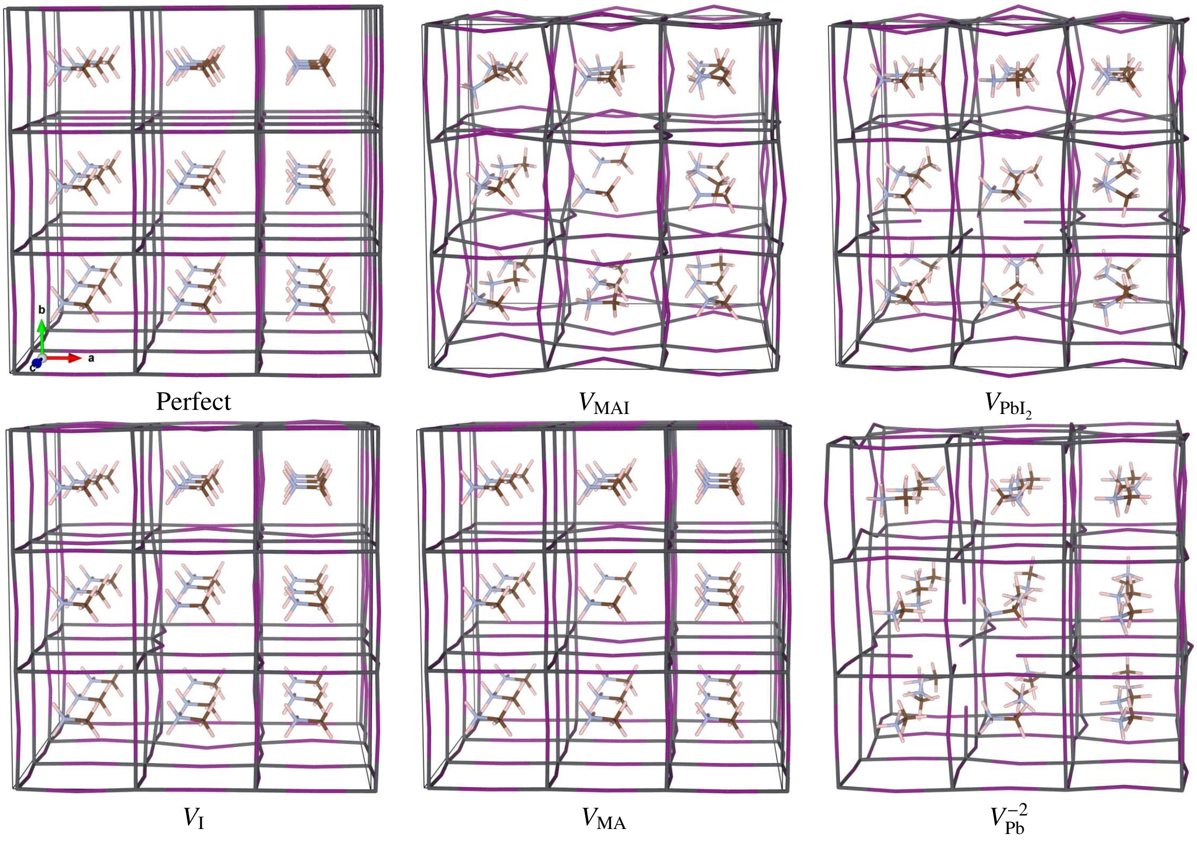


Figure S1. Optimized atomistic structures in $MAPbI_3$ and its vacancy-containing supercells.

*Corresponding author: Chol-Jun Yu, Email: ryongnam14@yahoo.com

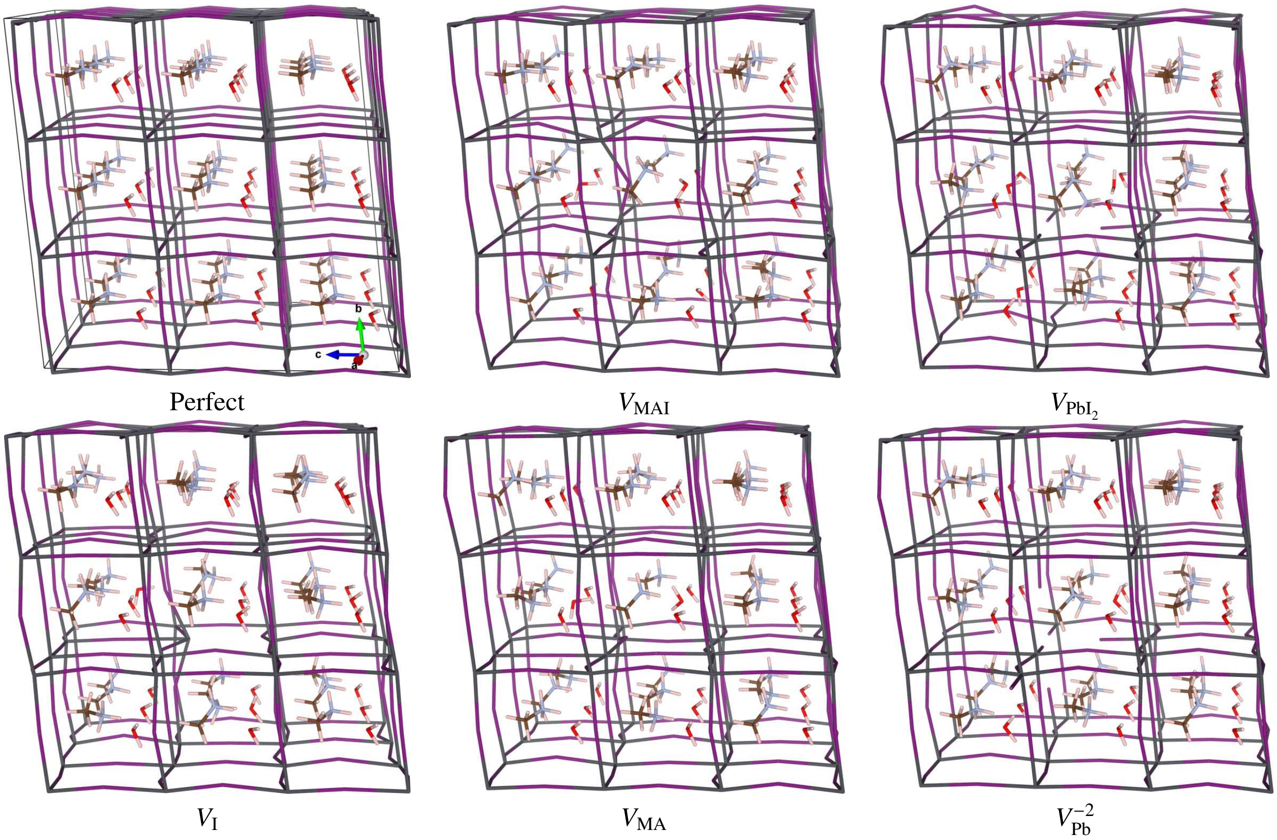


Figure S2. Optimized atomistic structures in $MAPbI_3\_H_2O$ and its vacancy-containing supercells.

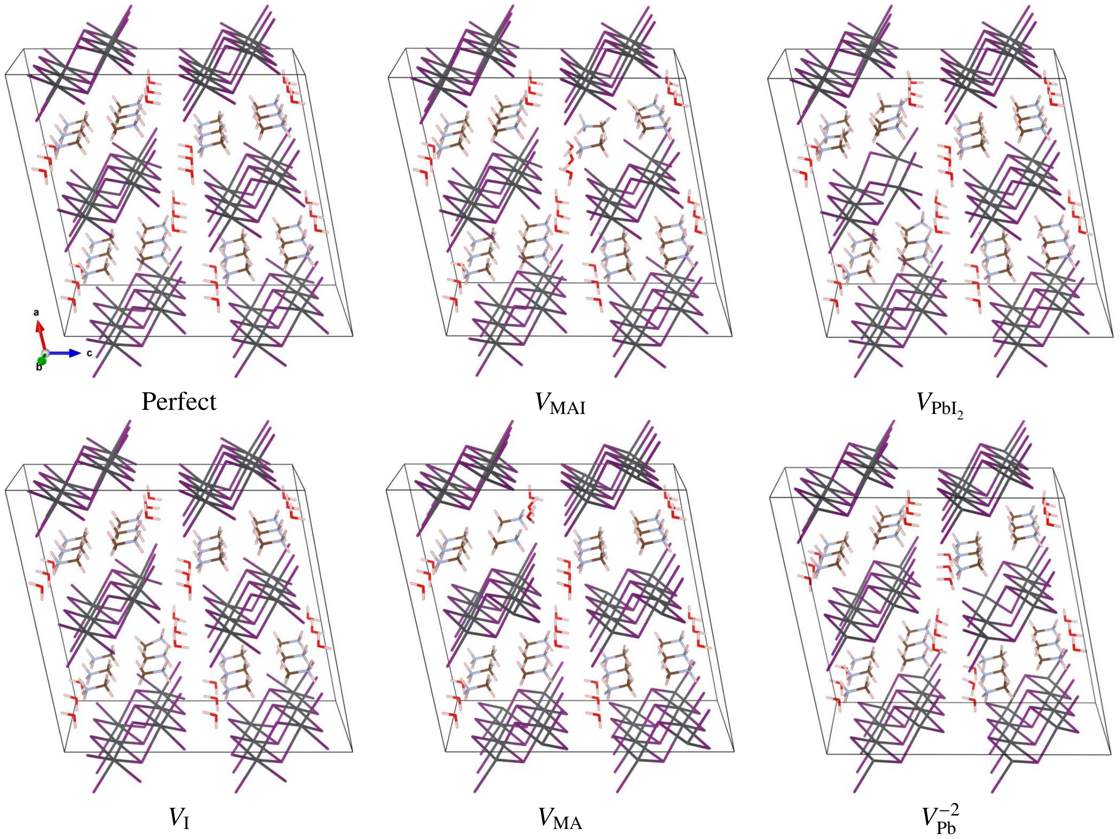


Figure S3. Optimized atomistic structures in $MAPbI_3 \cdot H_2O$ and its vacancy-containing supercells.

Table S1. Binding energy ($E_b$) of vacancy pair defects with different charge states in $MAPbI_3$, $MAPbI_3\_H_2O$ and $MAPbI_3 \cdot H_2O$.

| Species | Charge | Reaction | $E_b$ (eV) |
|---|---|---|---|
| | | $MAPbI_3$ | |
| MAI | 1+ | $V_{MA}^{0} + V_{I}^{+1} = V_{MAI}^{+1}$ | 1.313 |
| | 0 | $V_{MA}^{-1} + V_{I}^{+1} = V_{MAI}^{0}$ | 1.449 |
| | 1− | $V_{MA}^{-1} + V_{I}^{0} = V_{MAI}^{-1}$ | 1.193 |
| $PbI_2$ | 0 | $V_{Pb}^{-2} + 2V_{I}^{+1} = V_{PbI_2}^{0}$ | 0.944 |
| | 1− | $V_{Pb}^{-2} + V_{I}^{+1} + V_{I}^{0} = V_{PbI_2}^{-1}$ | 0.893 |
| | | $MAPbI_3\_H_2O$ | |
| MAI | 1+ | $V_{MA}^{0} + V_{I}^{+1} = V_{MAI}^{+1}$ | −0.392 |
| | 0 | $V_{MA}^{-1} + V_{I}^{+1} = V_{MAI}^{0}$ | −0.253 |
| | 1− | $V_{MA}^{-1} + V_{I}^{0} = V_{MAI}^{-1}$ | −0.018 |
| $PbI_2$ | 2+ | $V_{Pb}^{0} + 2V_{I}^{+1} = V_{PbI_2}^{+2}$ | −0.620 |
| | 1+ | $V_{Pb}^{-1} + 2V_{I}^{+1} = V_{PbI_2}^{+1}$ | −0.819 |
| | 0 | $V_{Pb}^{-2} + 2V_{I}^{+1} = V_{PbI_2}^{0}$ | 0.158 |
| | 1− | $V_{Pb}^{-2} + V_{I}^{+1} + V_{I}^{0} = V_{PbI_2}^{-1}$ | 0.030 |
| | | $MAPbI_3 \cdot H_2O$ | |
| MAI | 1+ | $V_{MA}^{0} + V_{I}^{+1} = V_{MAI}^{+1}$ | −0.513 |
| | 0 | $V_{MA}^{-1} + V_{I}^{+1} = V_{MAI}^{0}$ | −0.207 |
| | 1− | $V_{MA}^{-1} + V_{I}^{0} = V_{MAI}^{-1}$ | 0.029 |
| $PbI_2$ | 1+ | $V_{Pb}^{-1} + 2V_{I}^{+1} = V_{PbI_2}^{+1}$ | −0.224 |
| | 0 | $V_{Pb}^{-2} + 2V_{I}^{+1} = V_{PbI_2}^{0}$ | 0.282 |
| | 1− | $V_{Pb}^{-2} + V_{I}^{+1} + V_{I}^{0} = V_{PbI_2}^{-1}$ | −0.135 |
| | 2− | $V_{Pb}^{-2} + 2V_{I}^{0} = V_{PbI_2}^{-2}$ | −1.073 |

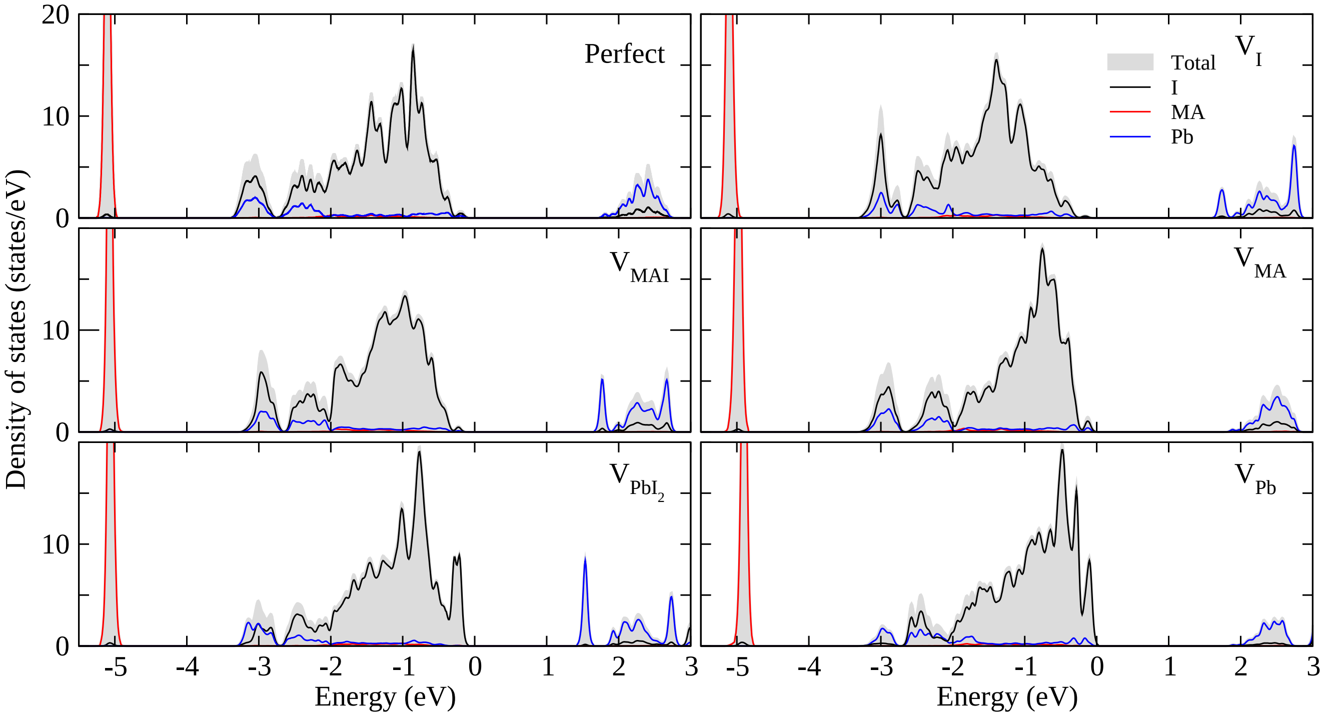


Figure S4. Atom-projected density of states in $MAPbI_3$ and its vacancy-containing phases.

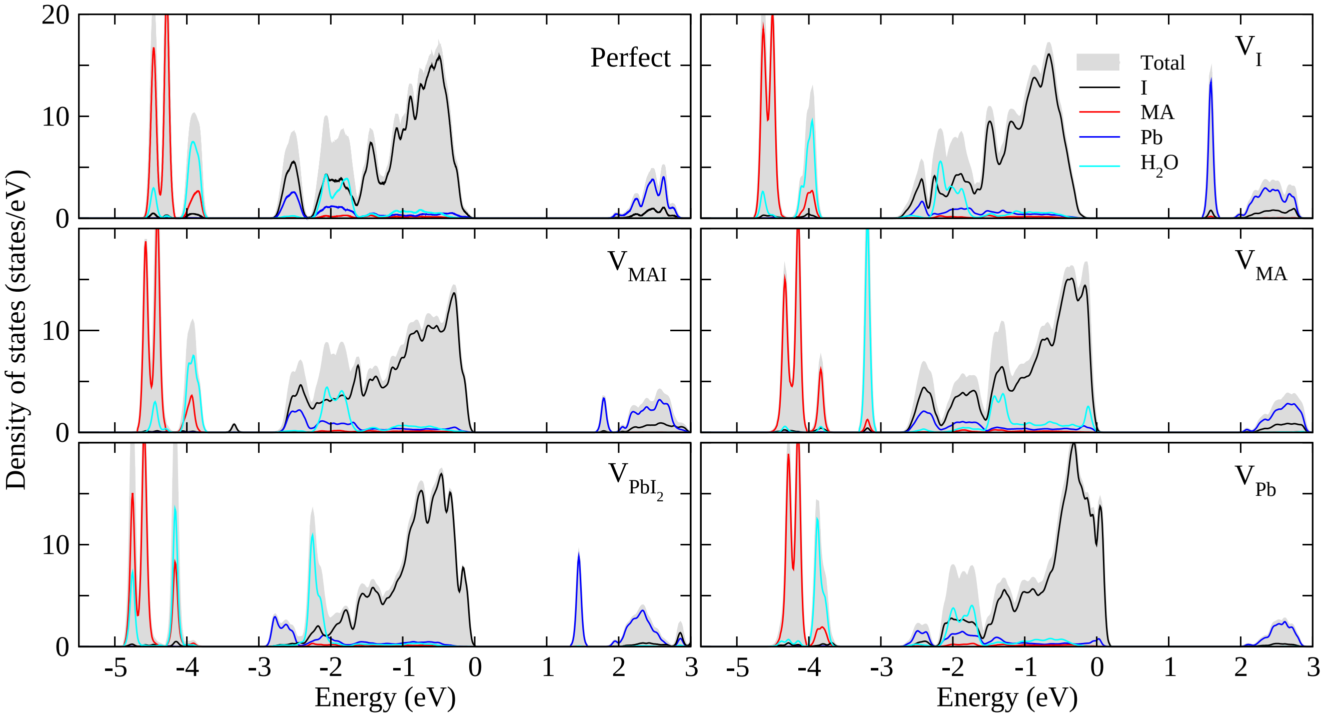


Figure S5. Atom-projected density of states in $MAPbI_3$_$H_2O$ and its vacancy-containing phases.

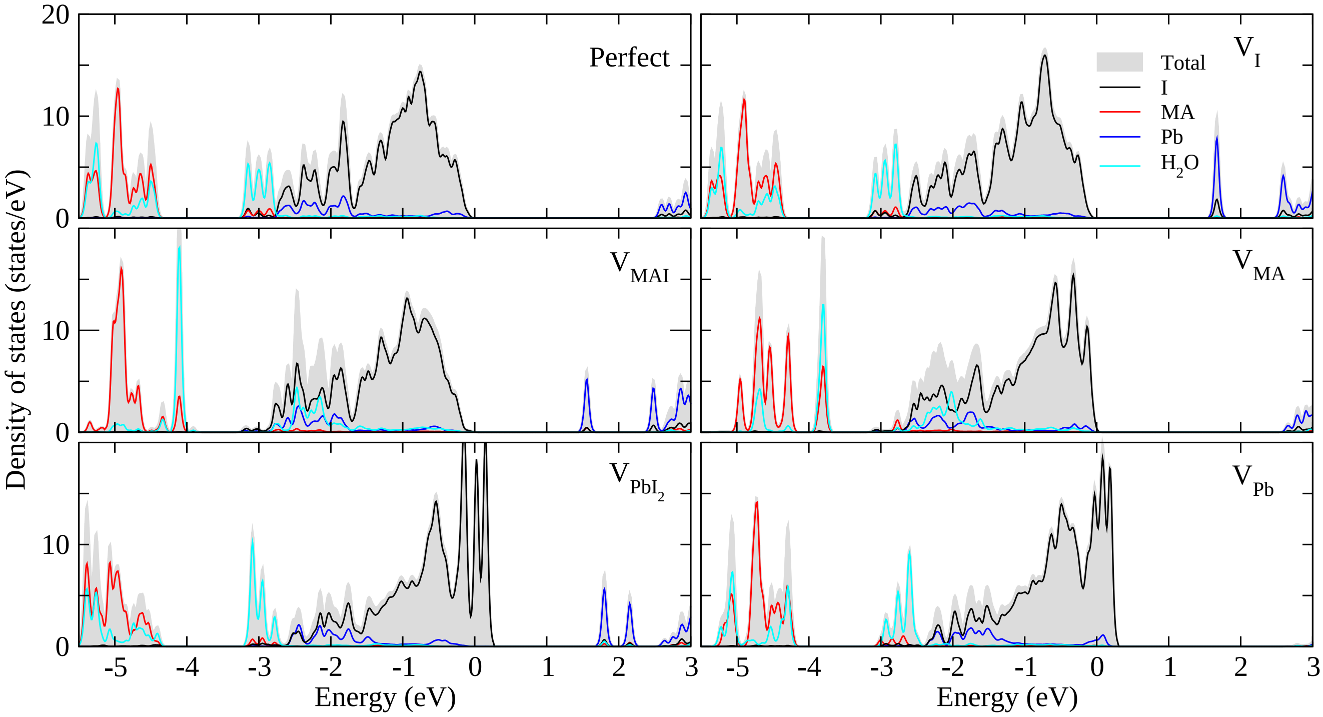


Figure S6. Atom-projected density of states in $MAPbI_3 \cdot H_2O$ and its vacancy-containing phases.
